# Supplementary material for: Meta-Learning Mini-Batch Risk Functionals
Source: arXiv:2301.11724 source file (2023-01-27)
Supplement: Supplementary file 1 [file 99_Appendix.tex]

\section{Pareto Plots}
\label{sec:paretoPlots}

\begin{figure*}[htb]
    \centering
    \subfloat[CVAR]{\label{fig:CVAR}\includegraphics[width=0.3\textwidth]{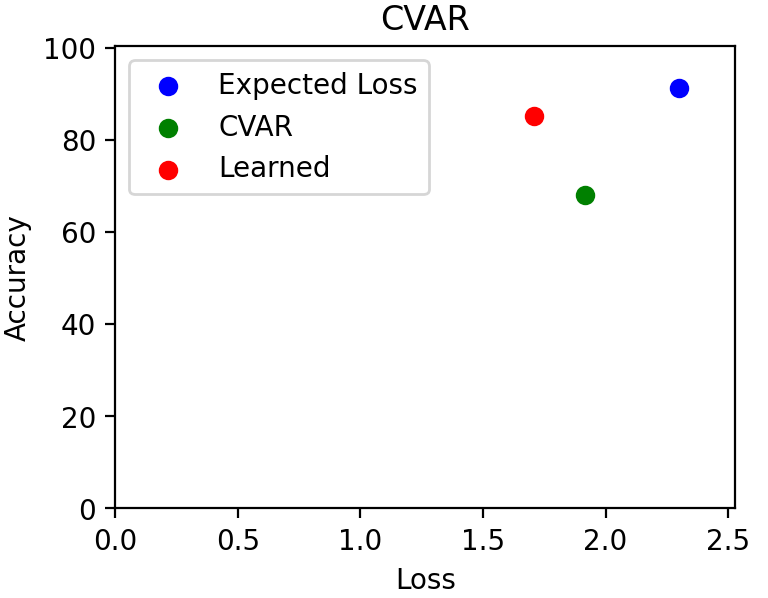}}
    \subfloat[ICVAR]{\label{fig:ICVAR}\includegraphics[width=0.3\textwidth]{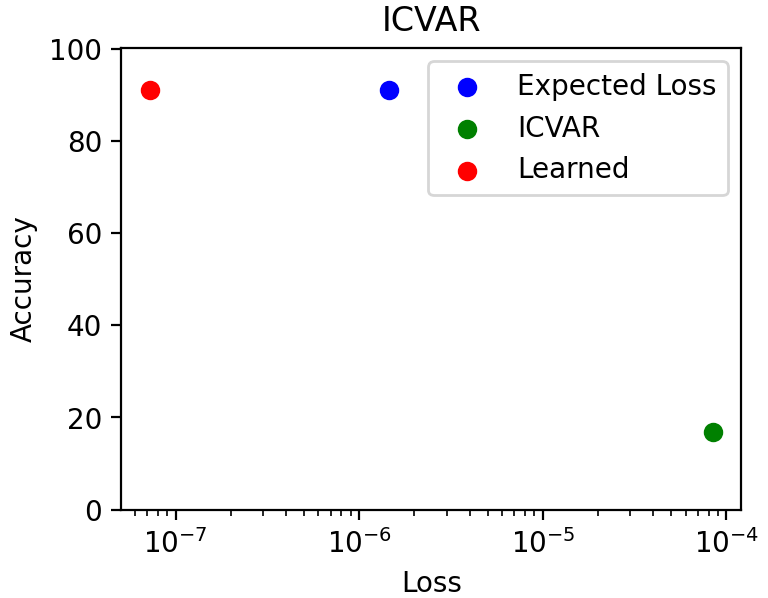}}
    \subfloat[Human]{\label{fig:human}\includegraphics[width=0.3\textwidth]{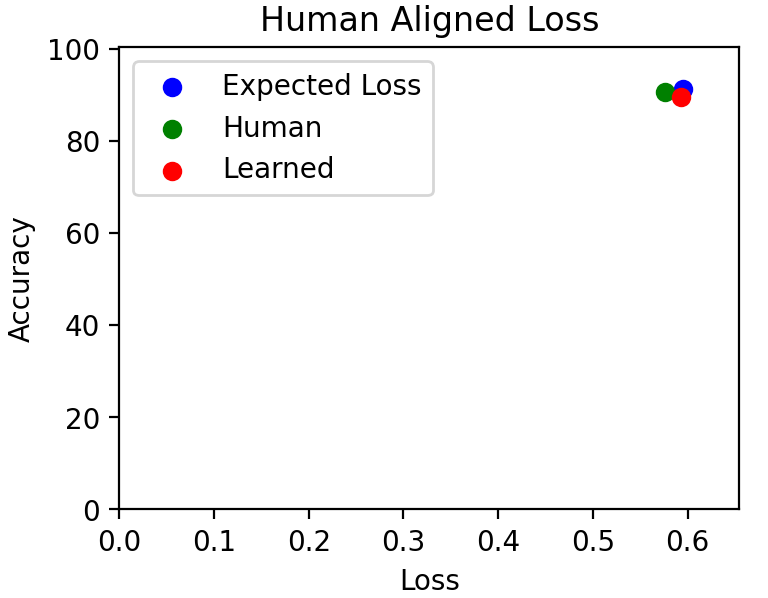}}
    \\
    \subfloat[Mean Variance]{\label{fig:meanv}\includegraphics[width=0.3\textwidth]{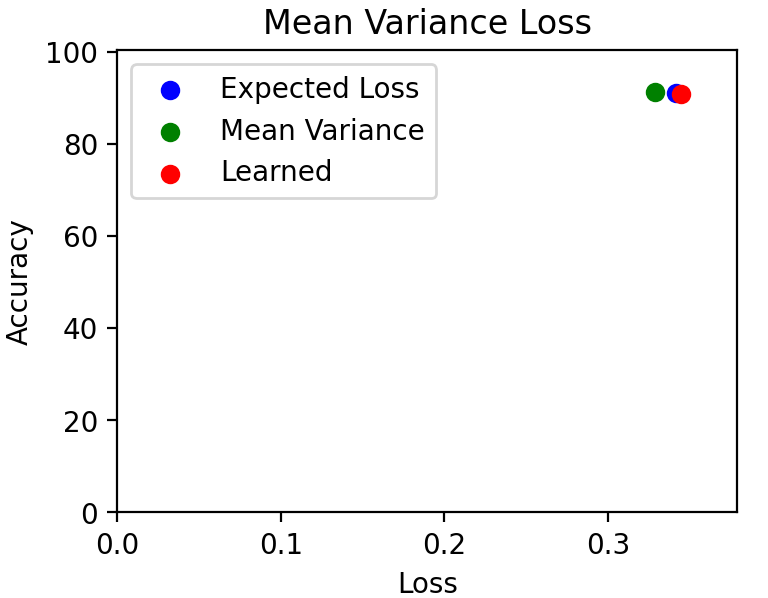}}
    \subfloat[Trimmed]{\label{fig:trimmed}\includegraphics[width=0.3\textwidth]{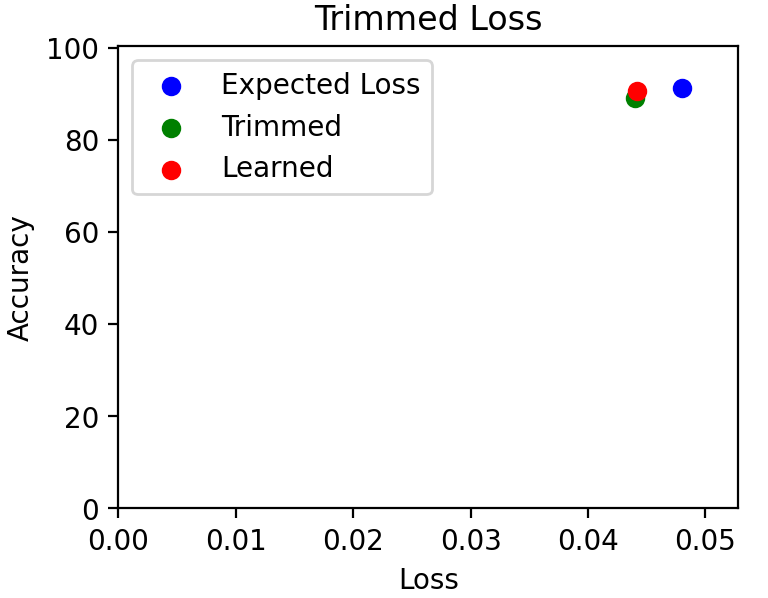}}
    \caption{Pareto Plots \hl{Update these!}}
    \label{fig:paretoPlots}
\end{figure*}

\section{Training with different levels of Label Noise}

\begin{table}[]
\centering
\caption{Learning risk functions for label noise.}
\label{tab:labelNoise}
\begin{tabular}{@{}lcc@{}}
\toprule
Noise & \begin{tabular}[c]{@{}c@{}}Expected\\ Value\end{tabular} & \begin{tabular}[c]{@{}c@{}}Learned \\ Risk Function\end{tabular} \\ \midrule
0\%   & \textbf{91.254 (0.2405)}                                 & \textbf{91.08 (0.2766)}                                          \\
5\%   & \textbf{80.62 (0.498)}                                   & \textbf{80.24 (1.054)}                                           \\
20\%  & 68.462 (0.3942)                                          & \textbf{77.43 (0.9506)}                                          \\
50\%  & 62.088 (2.201)                                           & \textbf{70.23 (1.2558)}                                          \\ \bottomrule
\end{tabular}
\end{table}

\section{Grid Search Info}
